# Supplementary material for: Nanocrystal Geometry Governs Phase Transformation Pathways in Palladium Hydride
Source: arXiv:2601.00093 ancillary file (2026-01-05)
Supplement: Supplementary file 1 [file SM_PdHxGeometry.pdf]

# Supporting Material for Nanocrystal Geometry Governs Phase Transformation Pathways in Palladium Hydride

## Supporting Figures

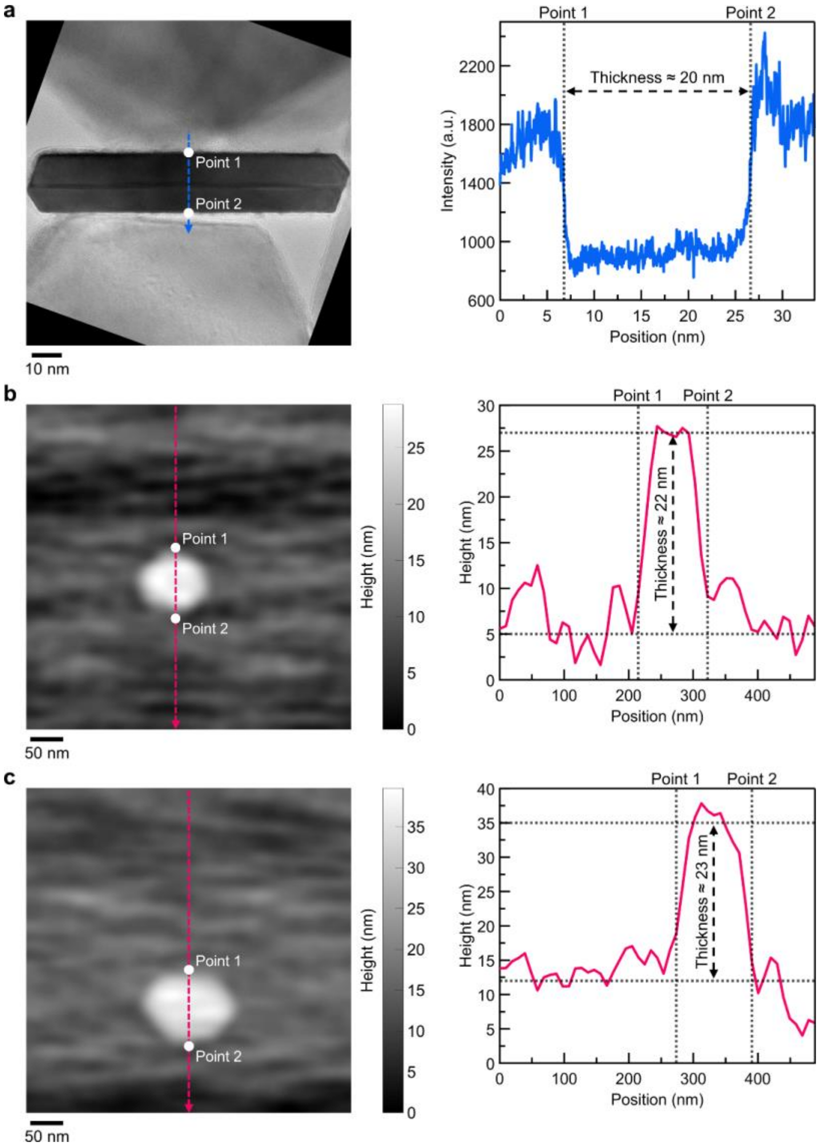


**Figure S1.** Thickness characterization of Pd nanoplates by HRTEM and AFM. **a**, Side-view HRTEM image of a representative Pd nanoplate with the corresponding intensity profile extracted along the dotted arrowed line. **b**,**c**, AFM topographic maps of other Pd nanoplates with height profiles extracted along the dotted arrowed lines. For each HRTEM and AFM image, 'Point 1' and 'Point 2' in the dotted lines correspond to the positions indicated in the associated intensity and height profiles, with arrows denoting the scan direction.

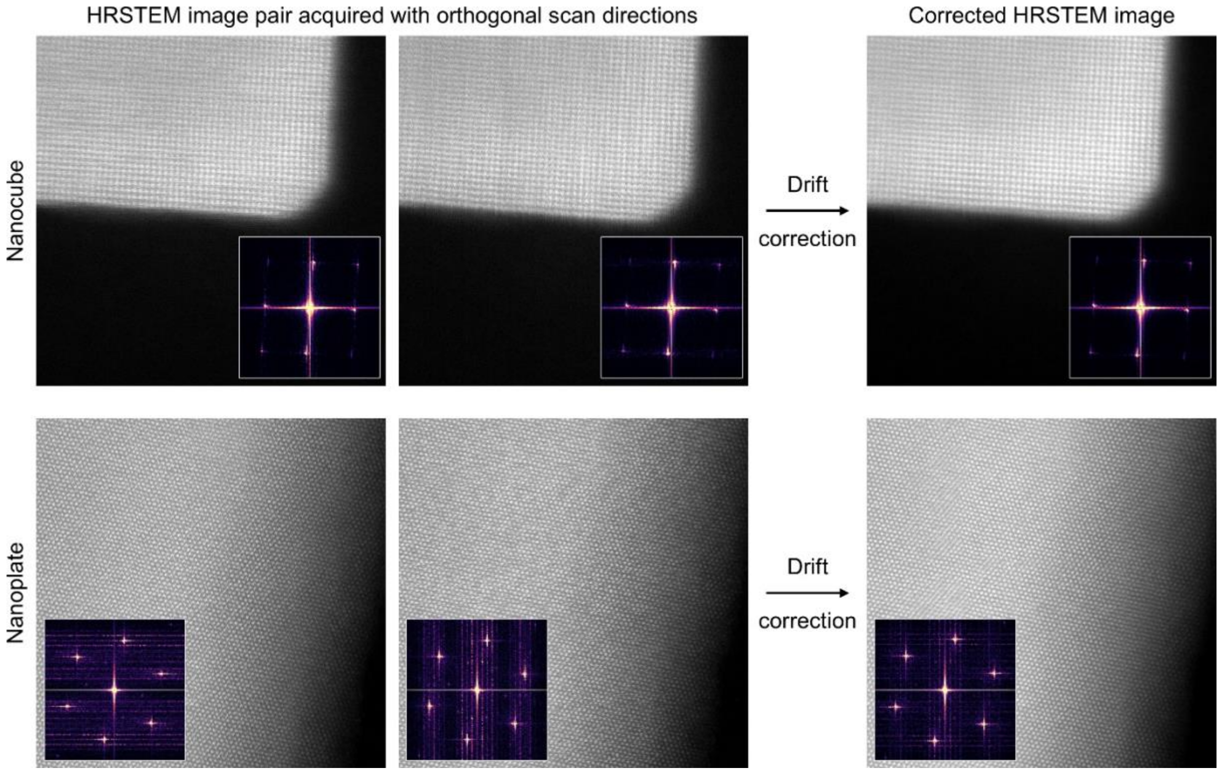


**Figure S2.** Post-acquisition drift correction of HRSTEM images. Raw image pairs (left) and drift-corrected images (right) of the nanocube and nanoplate shown in **Figure 1**, with corresponding FFT patterns displayed as insets. The HRSTEM images presented in **Figure 1** are cropped versions of the drift-corrected images.

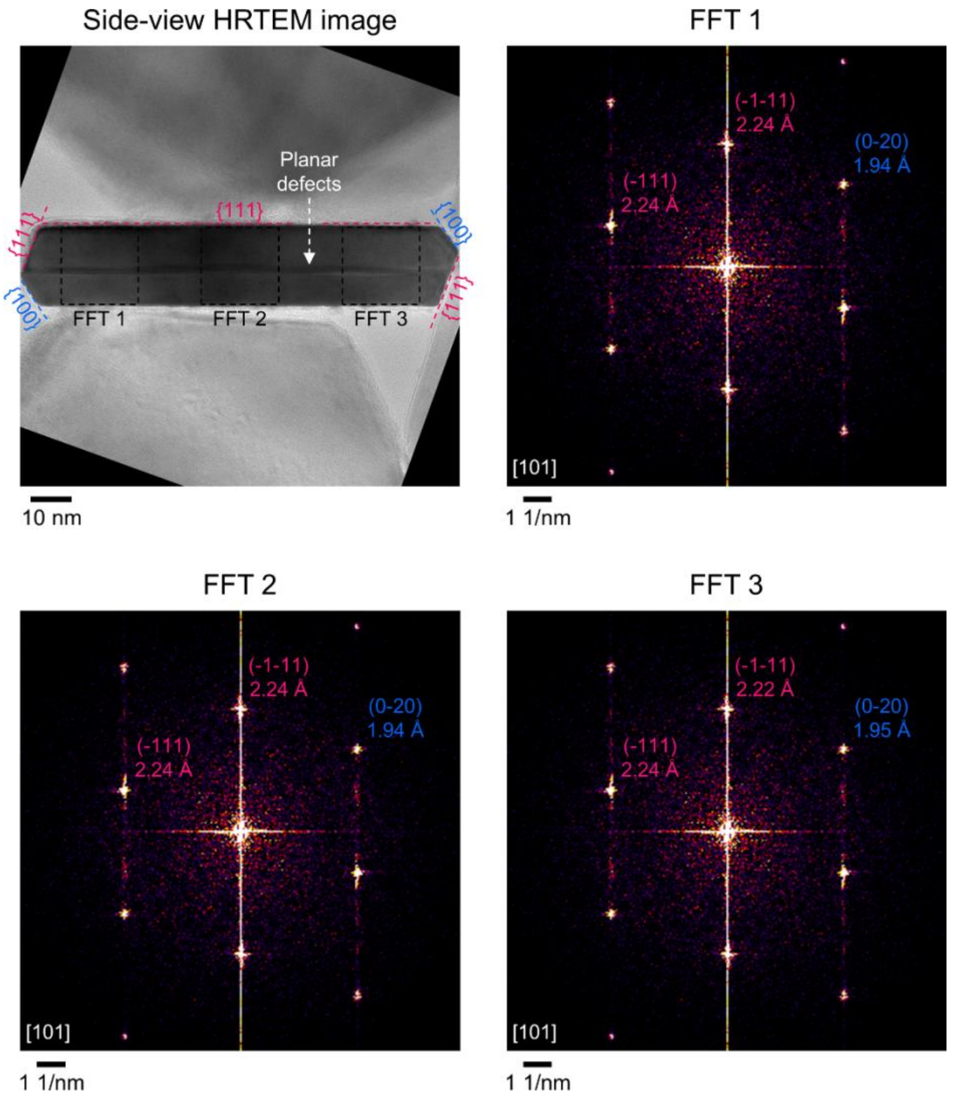


**Figure S3**. Crystallographic characteristics of the side facets of Pd nanoplates. The side-view HRTEM image shown in **Figure S1** is further analyzed here. FFT patterns are obtained from three boxed regions in the HRTEM image (labeled FFT 1–3) along the [101] zone axis. Crystallographic planes are assigned in the FFT patterns, with {200} planes marked in blue and {111} planes marked in pink. The analysis indicates that the top, bottom, and half of the shown side facets correspond to {111} planes, while the remaining side facets correspond to {100} planes. Planar defects lying on {111} planes are highlighted with a white dotted arrow in the HRTEM image; the vertical streaks observed in the FFT patterns suggest that stacking faults are the dominant defect type in this nanoplate.

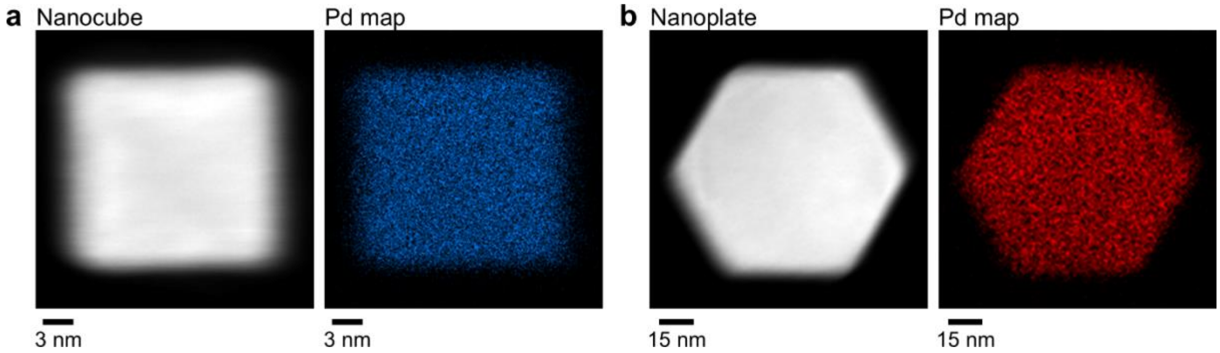


**Figure S4.** STEM and EDS characterization of Pd nanocrystals used in this study. **a**,**b**, STEM images (left) and corresponding Pd EDS elemental maps (right) of a representative Pd nanocube (**a**) and a Pd nanoplate (**b**).

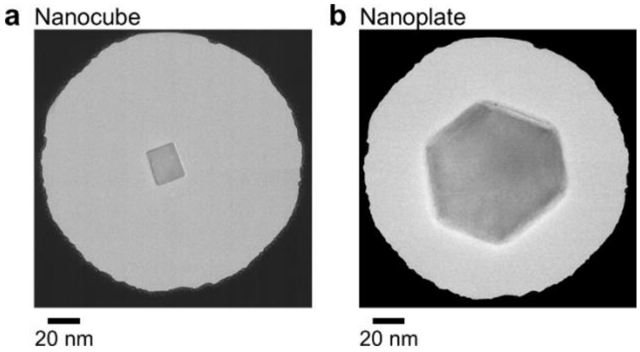


**Figure S5.** Pd nanocrystals used for the HRTEM and SAED analyses. **a**,**b**, TEM images of the Pd nanocube (**a**) and the Pd nanoplate (**b**) used to acquire the HRTEM images and SAED patterns shown in **Figure 1**. The selected area aperture encompasses the nanocrystals in each image. The HRTEM image and SAED pattern for the Pd nanocube in **Figure 1** were rotated to enhance visual clarity.

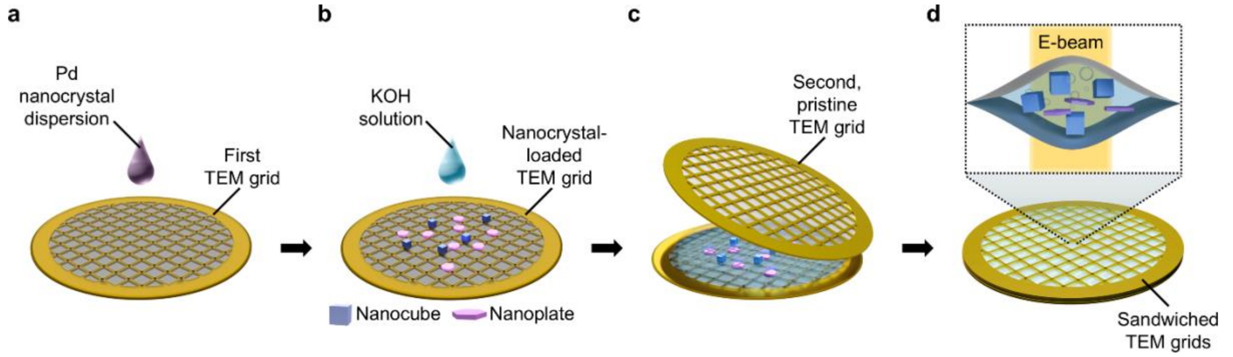


**Figure S6.** Schematic illustration of the experimental procedure for assembling liquid cells. **a**, Dispersion of Pd nanocrystals (nanocubes or nanoplates) is drop-cast onto a carbon film supported on a TEM grid, resulting in the deposition of nanocrystals on the first TEM grid. **b**, A droplet of aqueous KOH solution is then drop-cast onto the nanocrystal-loaded TEM grid. **c**, A second pristine carbon-film-coated TEM grid is placed on top, sandwiching the KOH solution and Pd nanocrystals to form a carbon-film-based liquid cell. **d**, Under electron-beam (E-beam) irradiation, radiolysis of the encapsulated aqueous solution generates hydrogen *in situ*, enabling the hydrogenation of the encapsulated Pd nanocrystals.

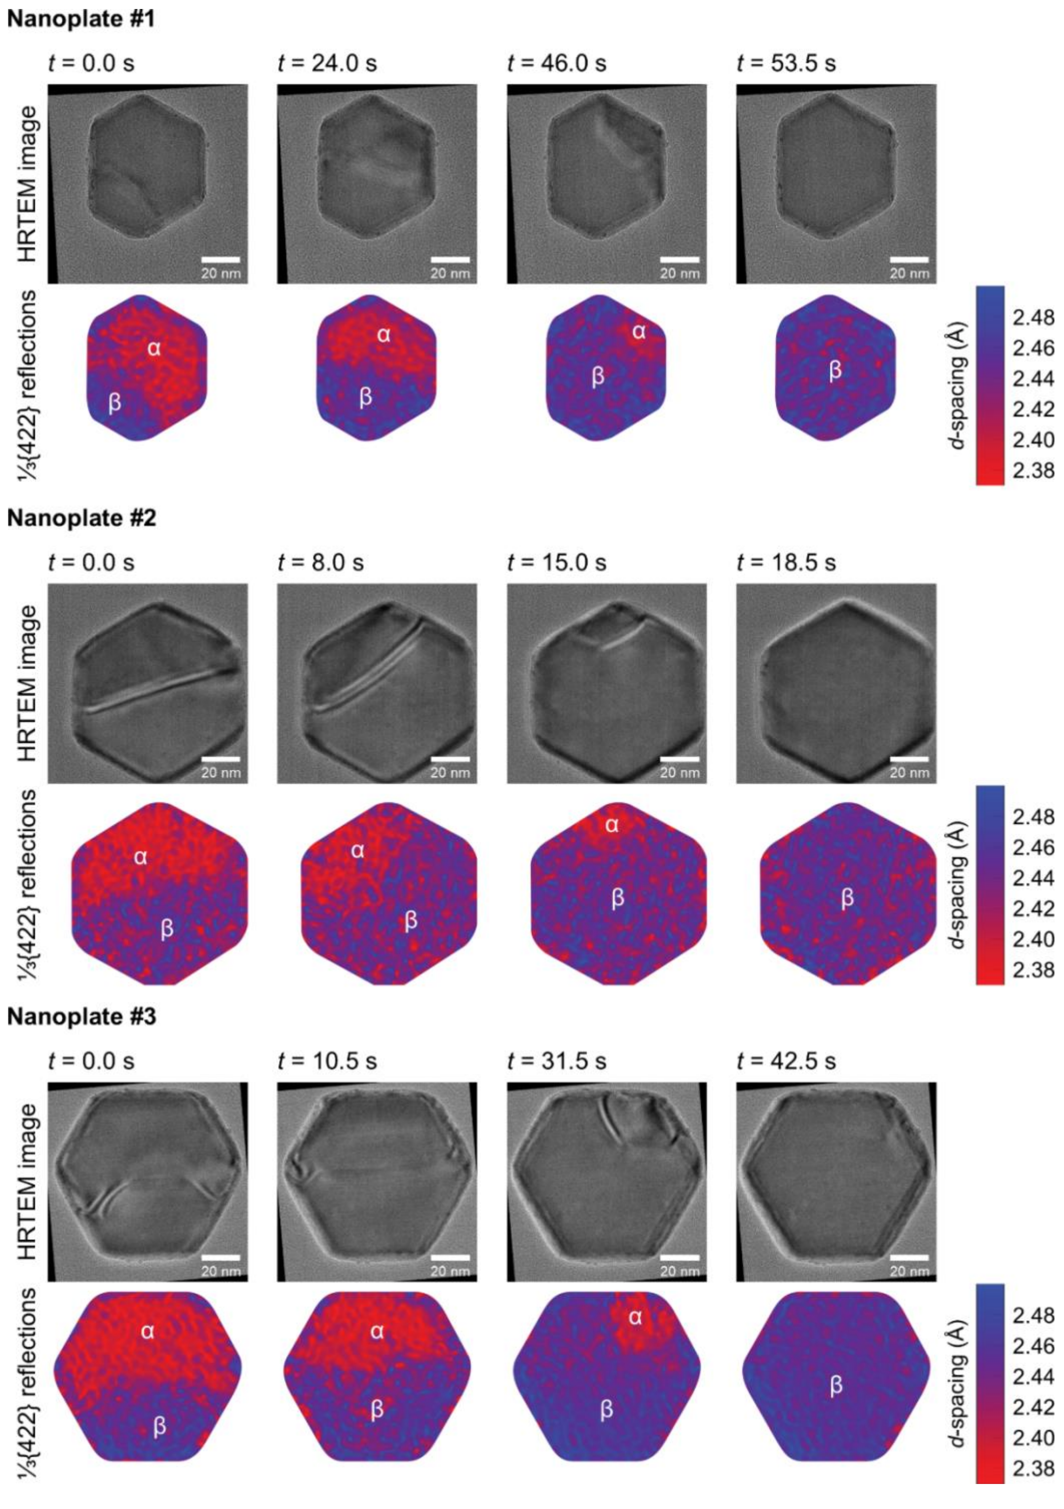


**Figure S7.** Amplitude-weighted ⅓{422} *d*-spacing colormaps for $PdH_x$ Nanoplates, obtained from the *in situ* HRTEM image sequences in **Figure 2**. Colormaps derived from both {220} and defect-induced ⅓{422} reflections reveal qualitatively consistent evolution of α- and β-$PdH_x$ phase distributions.

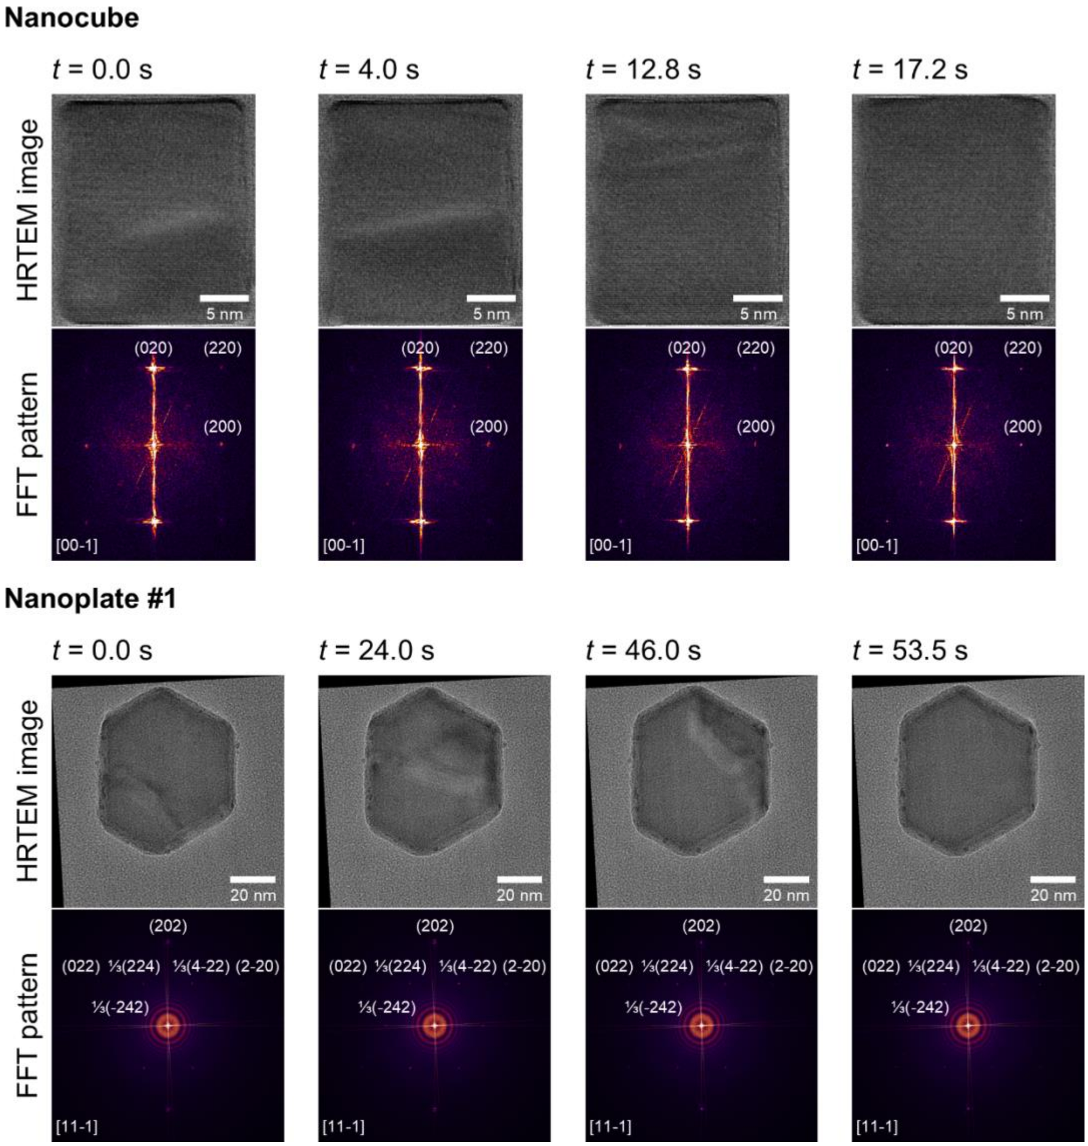


**Figure S8.** FFT patterns derived from the corresponding *in situ* HRTEM image sequences of $PdH_x$ nanocrystals shown in **Figure 2**. The nanocube is oriented along the [00-1] zone axis, whereas the nanoplate is oriented along the [11-1] zone axis. The FFT patterns display the crystallographic reflections used to generate the *d*-spacing colormaps: {200} for the nanocube and {220} together with forbidden ⅓{422} for the nanoplate.

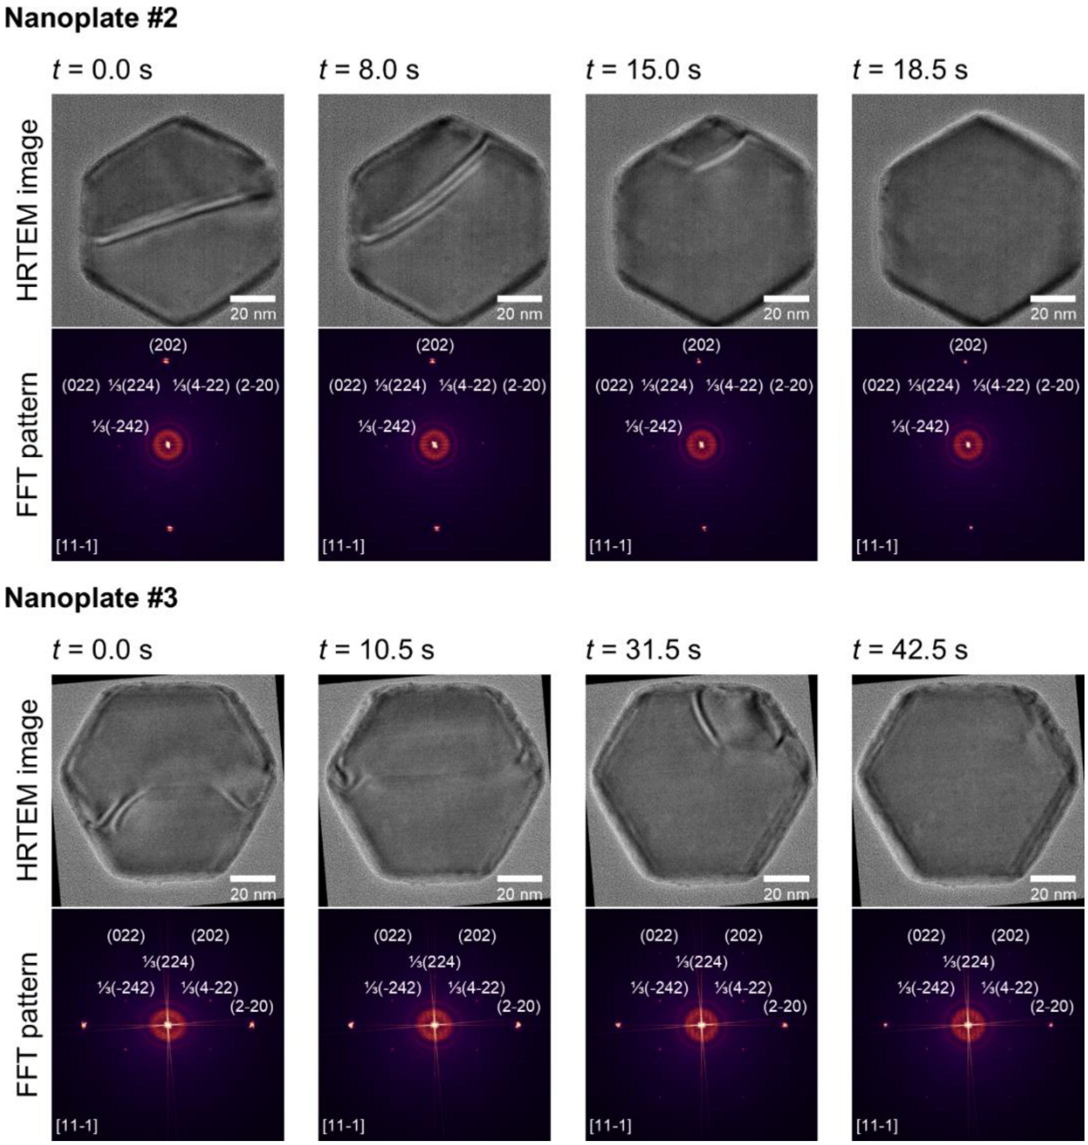


**Figure S9.** FFT patterns derived from the corresponding *in situ* HRTEM image sequences of $PdH_x$ nanocrystals shown in **Figure 2**. The nanoplates are oriented along the [11-1] zone axis. The FFT patterns display the crystallographic reflections used to generate the *d*-spacing colormaps: {220} together with forbidden ⅓{422} for the nanoplates.

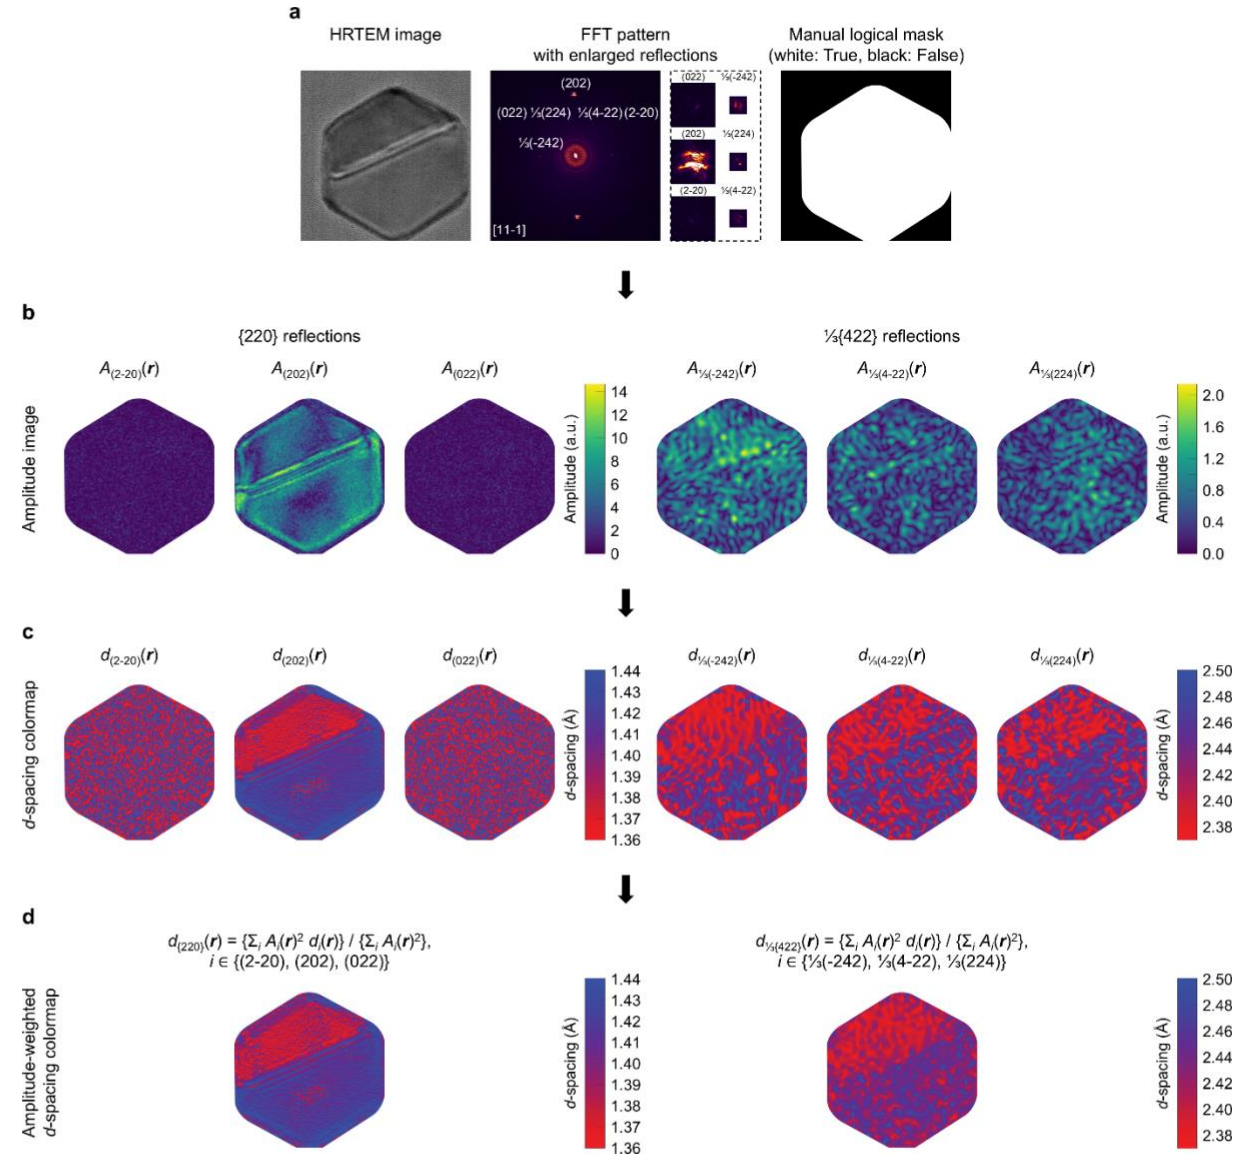


**Figure S10.** Workflow for generating amplitude-weighted $d$-spacing colormaps from an HRTEM image. **a**, Representative HRTEM image of Nanoplate #2, its FFT pattern along the [11-1] zone axis with enlarged views of selected {220} and ⅓{422} reflections, and a manual logical mask (white: True, black: False) used to isolate the nanocrystal region. **b**, Amplitude images $A_g(\boldsymbol{r})$ of selected Bragg reflections, obtained as the modulus of the inverse Fourier transform of the Bragg-filtered Fourier transform of the HRTEM image, $H'_g(\boldsymbol{r})$: (2-20), (202), (022) for the {220} family and ⅓(-242), ⅓(4-22), ⅓(224) for the ⅓{422} family. **c**, $d$-spacing colormaps $d_g(\boldsymbol{r})$ obtained from strain maps $\varepsilon_g(\boldsymbol{r})$ relative to the reference lattice vector $\boldsymbol{g}$ of the corresponding Bragg reflections. **d**, Final amplitude-weighted $d$-spacing colormaps $d_{\{220\}}(\boldsymbol{r})$ and $d_{⅓\{422\}}(\boldsymbol{r})$, generated by weighting each $d_g(\boldsymbol{r})$ by the squared amplitude image $A_g(\boldsymbol{r})^2$ and summing over the selected reflections.

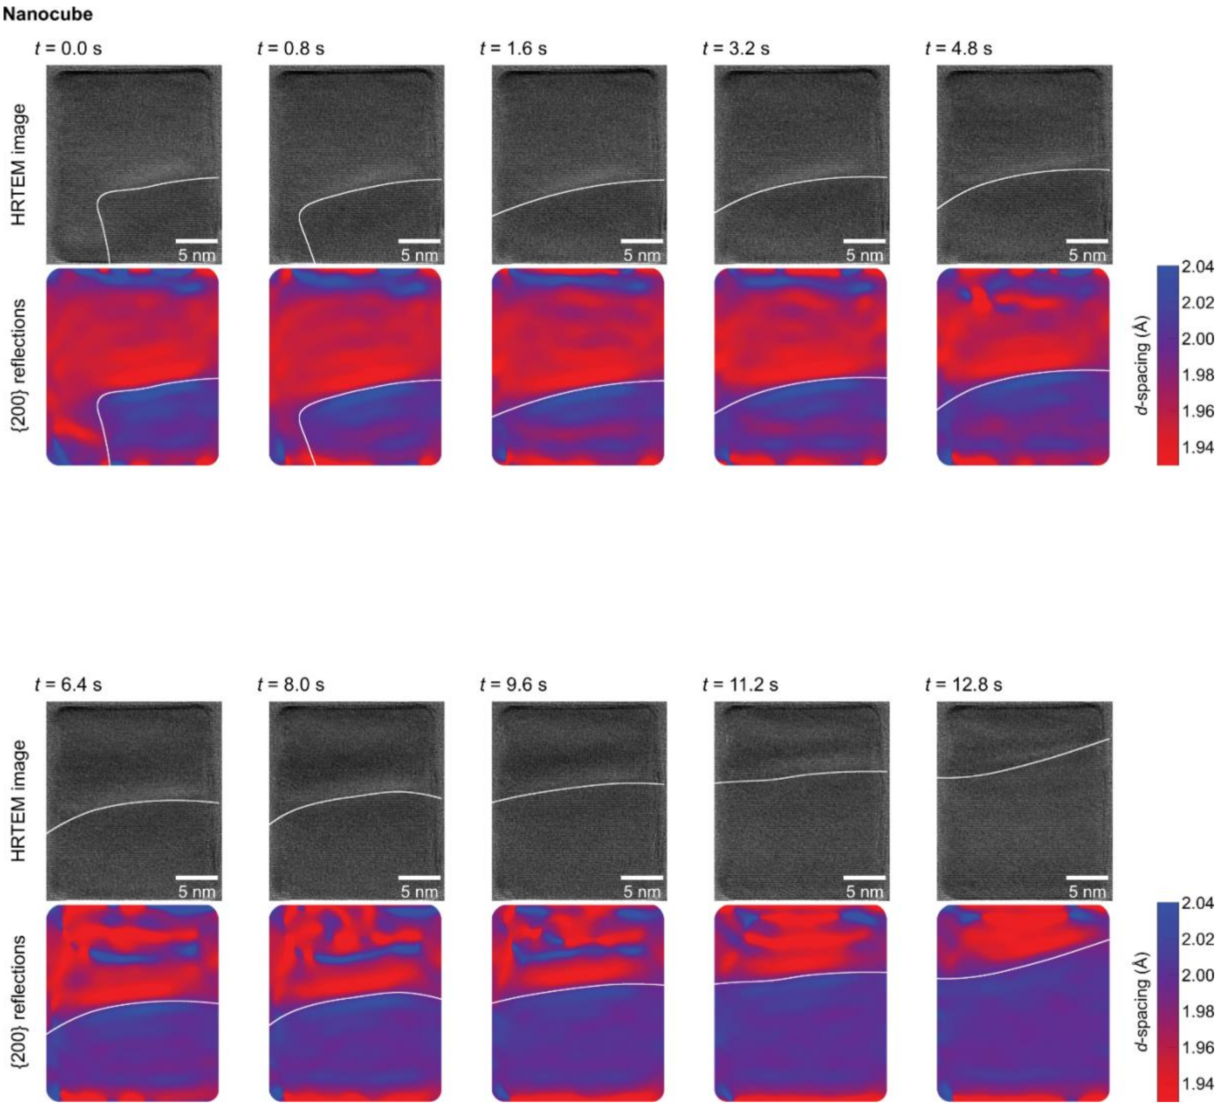


**Figure S11.** α/β-$PdH_x$ interphase boundary contour extraction in Nanocube. Representative sequential HRTEM images (top) and corresponding amplitude-weighted {200} *d*-spacing colormaps (bottom), providing the structural basis for identifying and manually tracing the α/β-$PdH_x$ interface contours shown in **Figure 3a**. The traced interphase boundaries are displayed as solid white lines superimposed on both the HRTEM images and the *d*-spacing colormaps.

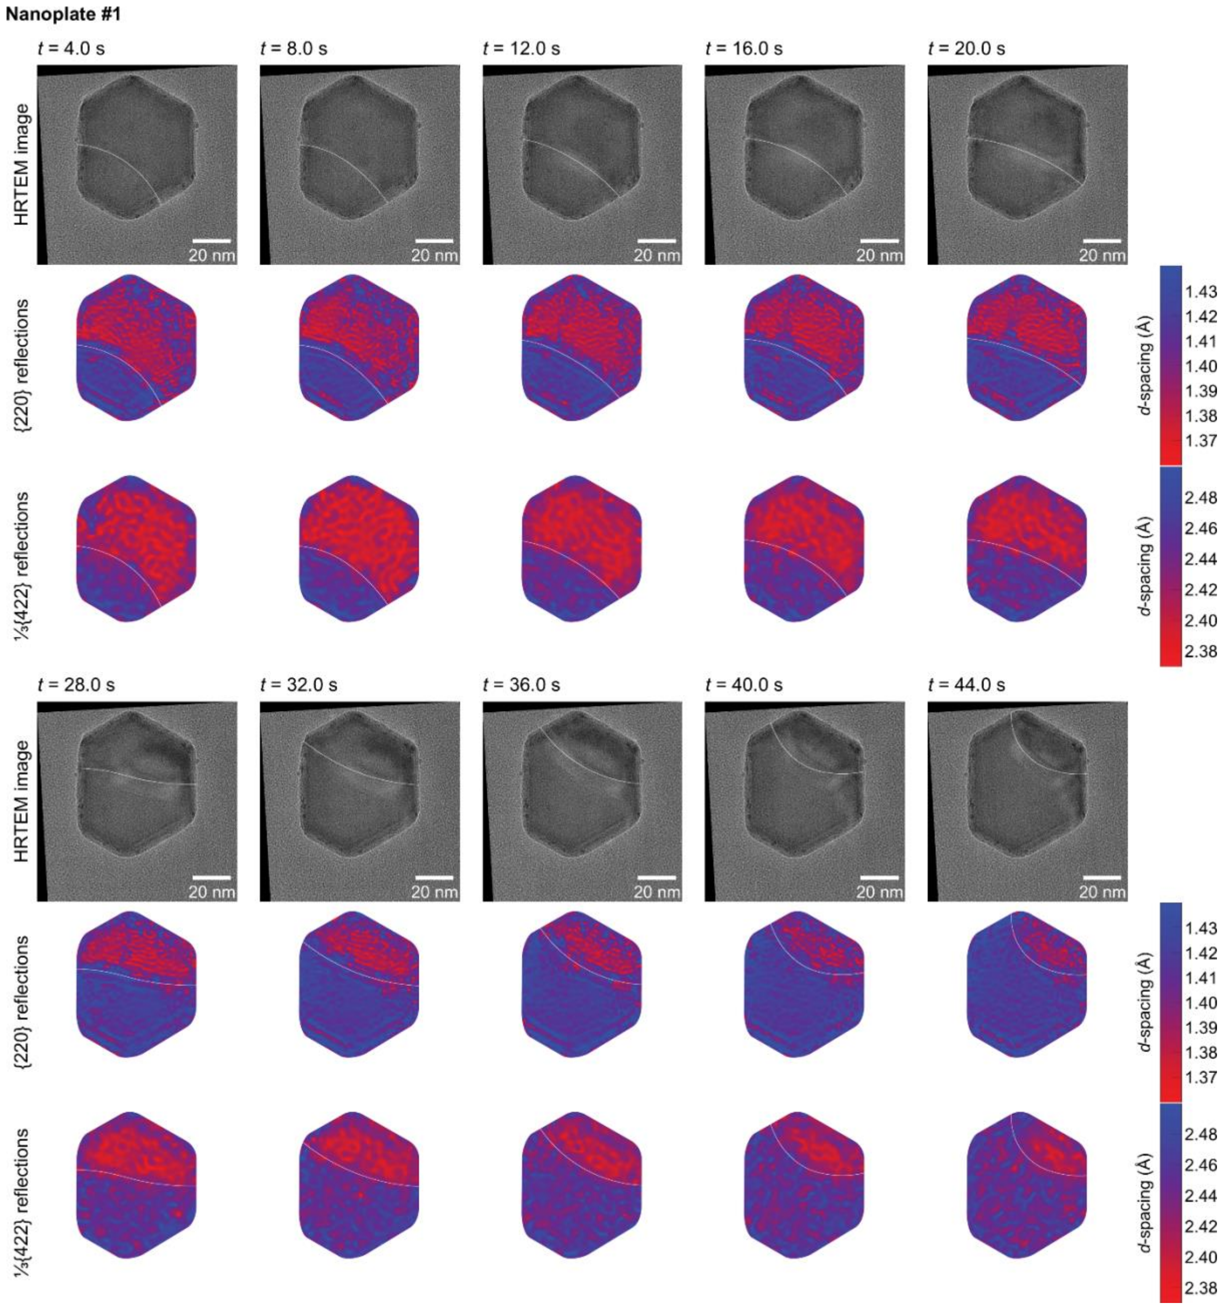


**Figure S12.** α/β-Pd$H_x$ interphase boundary contour extraction in Nanoplate #1. Representative sequential HRTEM images (top) and corresponding amplitude-weighted {220} and ⅓{422} *d*-spacing colormaps (bottom), providing the structural basis for identifying and manually tracing the α/β-Pd$H_x$ interface contours shown in **Figure 3b**. The traced interphase boundaries are displayed as solid white lines superimposed on both the HRTEM images and the *d*-spacing colormaps.

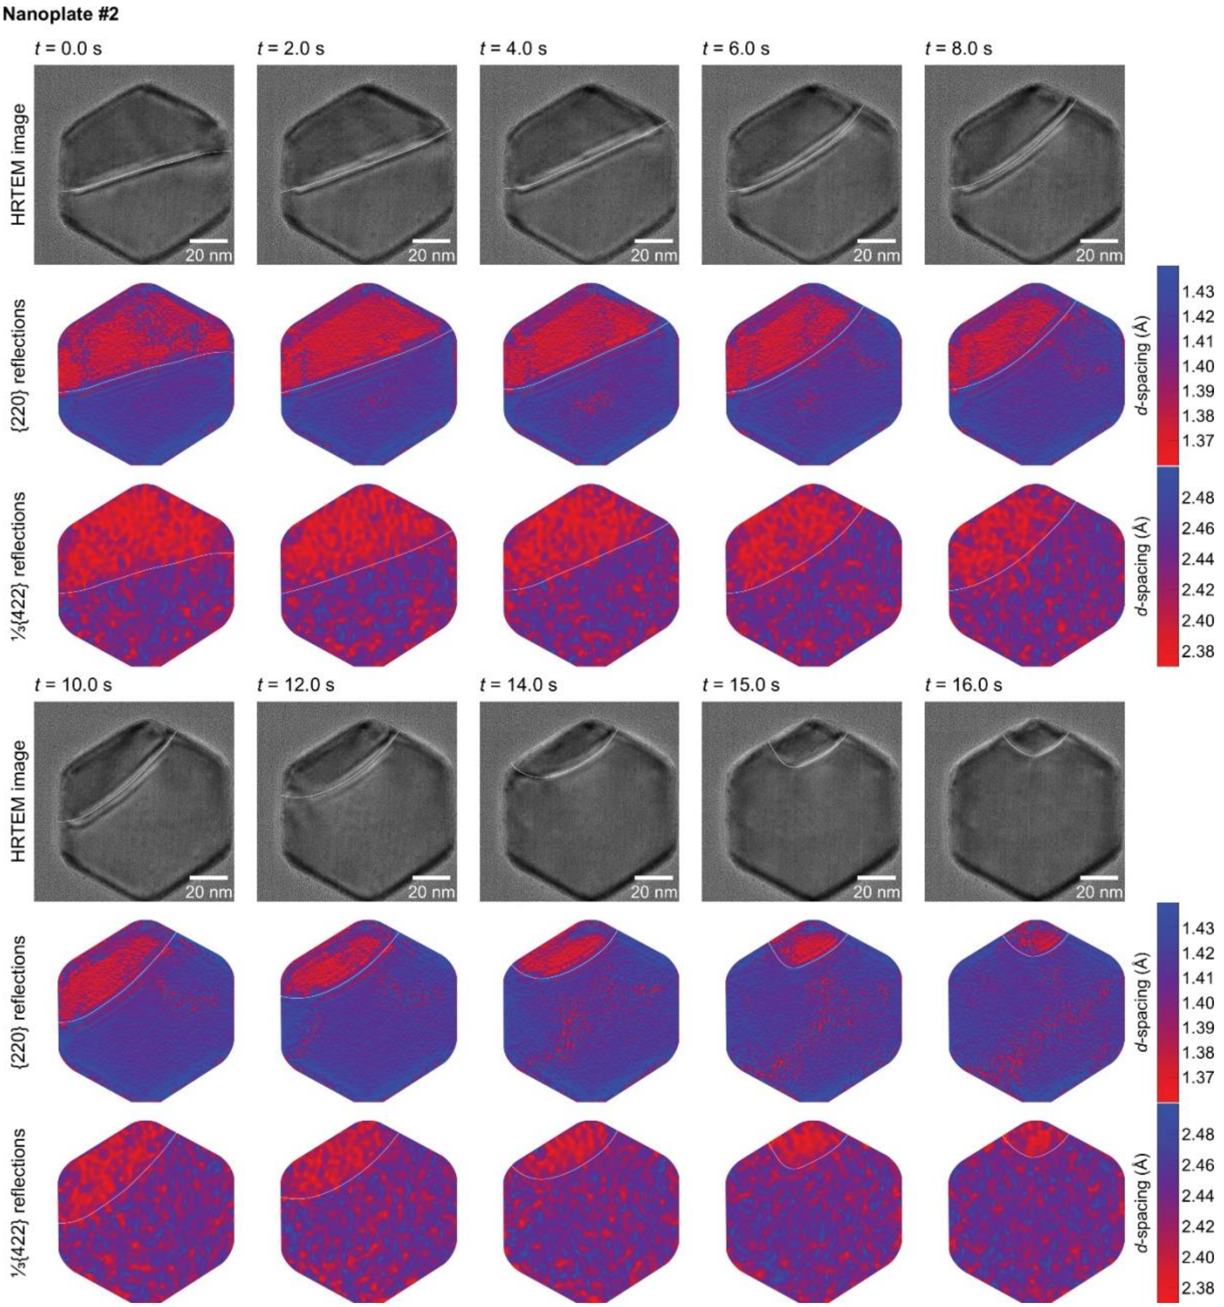


**Figure S13.** α/β-$PdH_x$ interphase boundary contour extraction in Nanoplate #2. Representative sequential HRTEM images (top) and corresponding amplitude-weighted {220} and ⅓{422} *d*-spacing colormaps (bottom), providing the structural basis for identifying and manually tracing the α/β-$PdH_x$ interface contours shown in **Figure 3c**. The traced interphase boundaries are displayed as solid white lines superimposed on both the HRTEM images and the *d*-spacing colormaps.

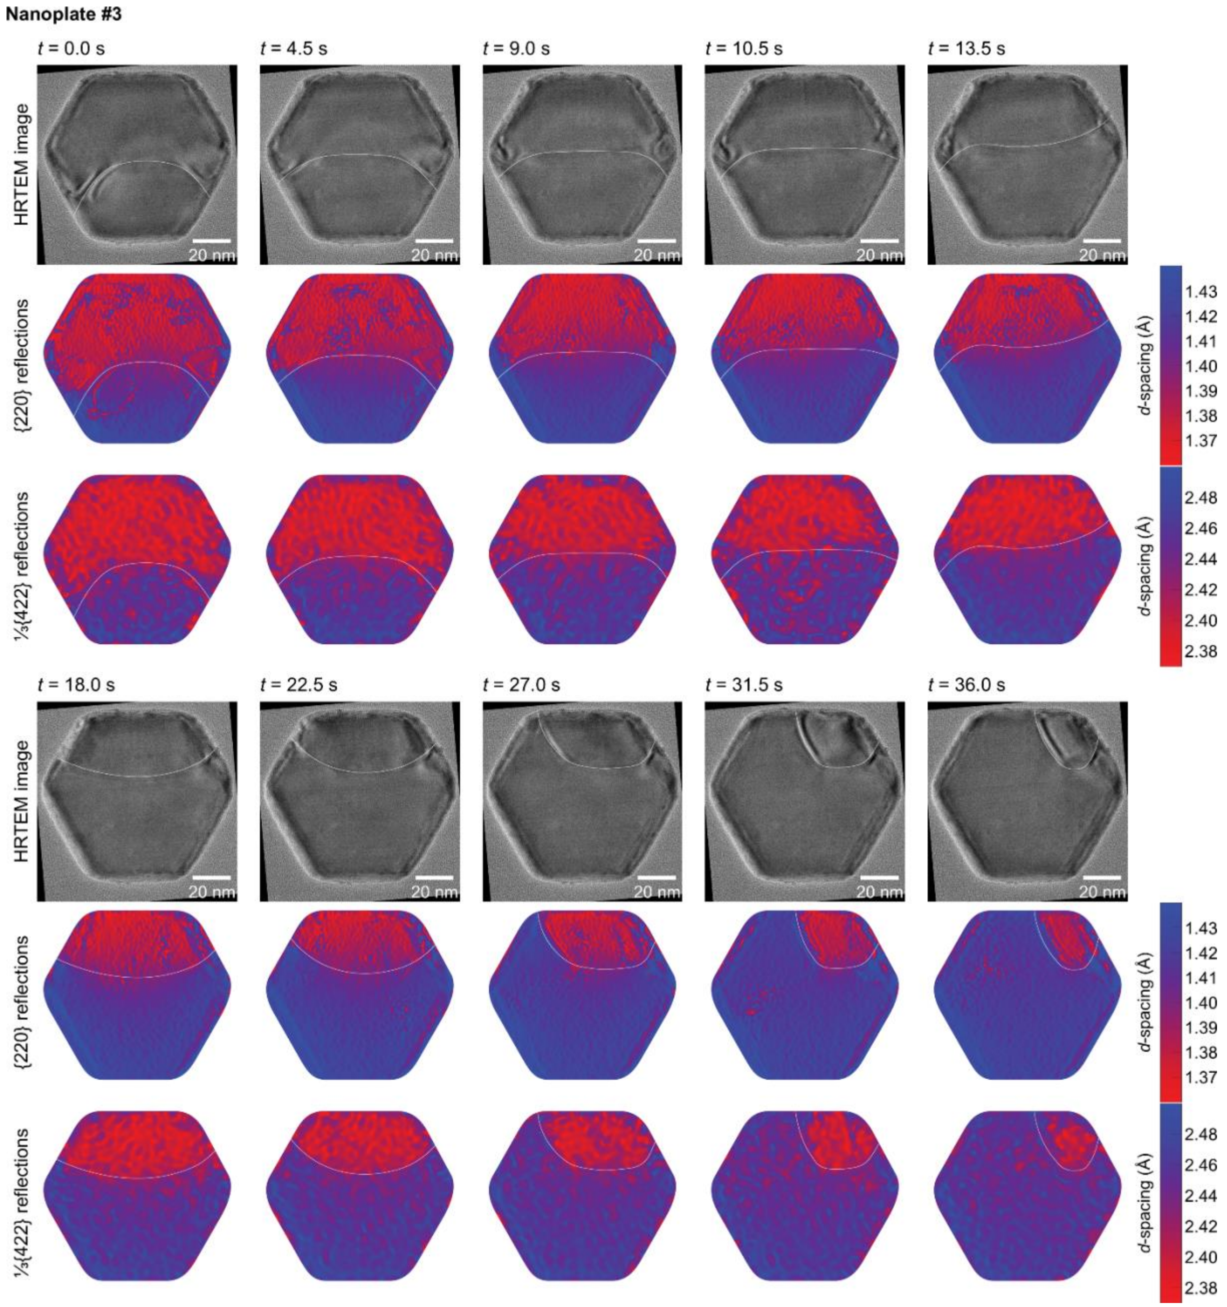


**Figure S14.** α/β-Pd$H_x$ interphase boundary contour extraction in Nanoplate #3. Representative sequential HRTEM images (top) and corresponding amplitude-weighted {220} and ⅓{422} *d*-spacing colormaps (bottom), providing the structural basis for identifying and manually tracing the α/β-Pd$H_x$ interface contours shown in **Figure 3d**. The traced interphase boundaries are displayed as solid white lines superimposed on both the HRTEM images and the *d*-spacing colormaps.

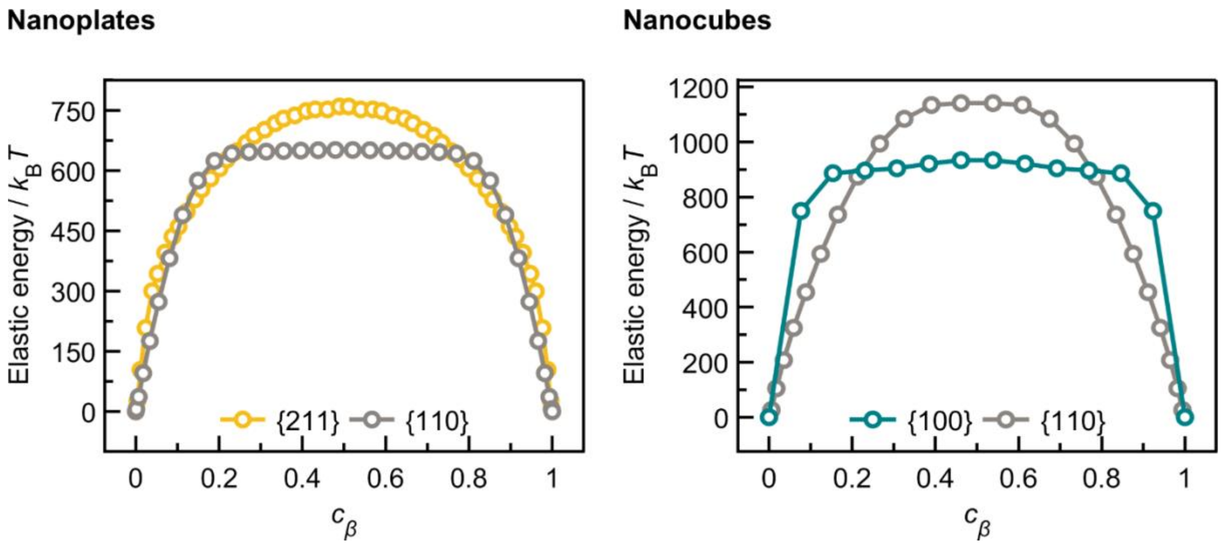


**Figure S15.** The elastic energy of idealized, perfectly flat α/β-$PdH_x$ interfaces in the nanoplates and nanocubes, plotted as a function of the β-phase fraction ($c_\beta$). Note that the elastic-energy crossovers between the two crystallographic orientations in both geometries occur at different $c_\beta$ values than in **Figure 4b** and **5b**. This difference arises because, in the dynamical simulations, the true interface is curved and not perfectly aligned with a single crystallographic orientation at $c_\beta$ values away from 0.5 (**Figure 4c**, **5c**, and **S17–S19**). The most relevant feature for the analysis in the main text is the difference in elastic energy at $c_\beta = 0.5$.

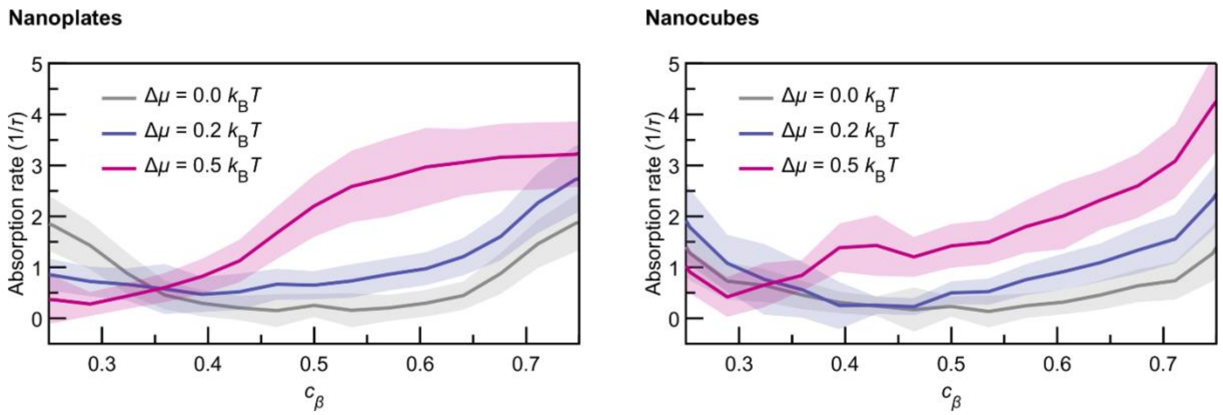


**Figure S16.** The average absorption rate in the nanoplates and nanocubes plotted against the β-phase fraction. The absorption rate is defined as the rate of change in the number of β-phase sites, measured in units of the fundamental simulation time (see **Methods**).

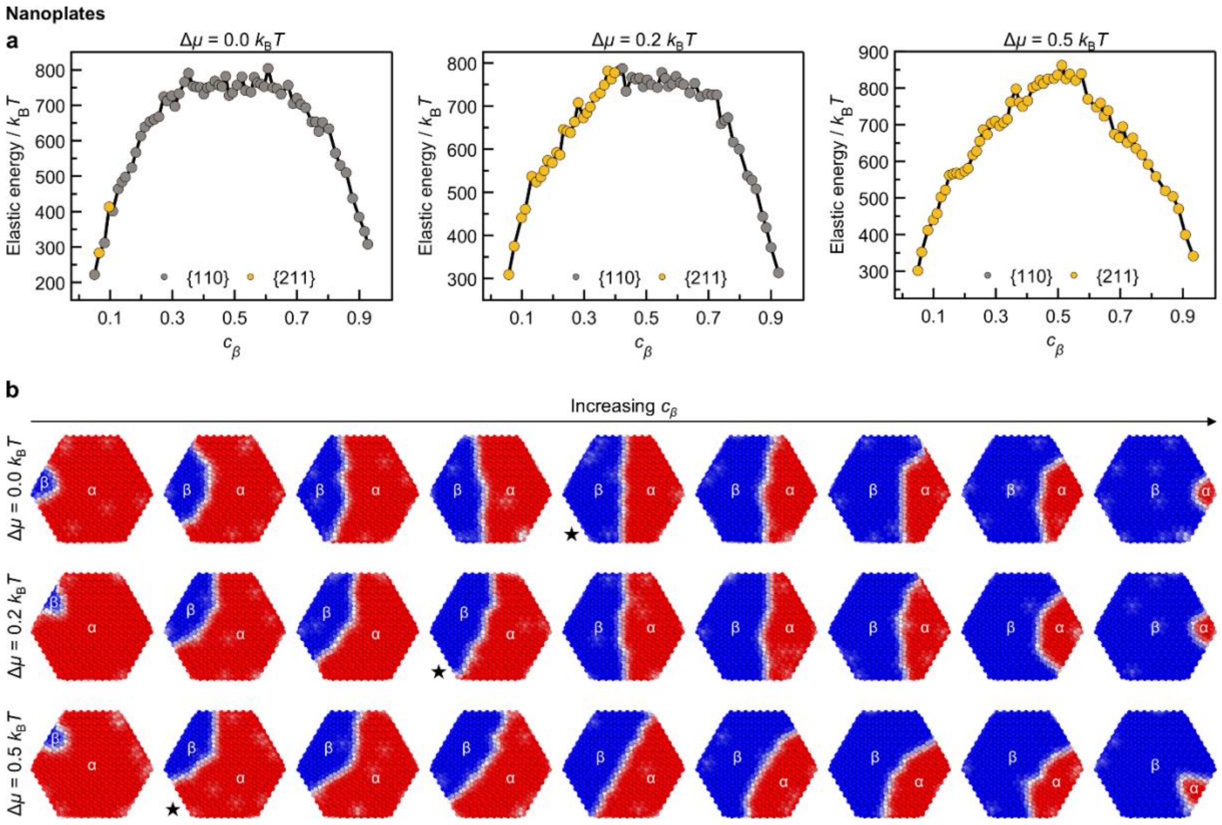


**Figure S17.** Detailed analysis of the representative hydrogenation trajectories in nanoplates. **a**, For each representative trajectory under the three chemical driving forces, $\Delta\mu$, the elastic energy (see **Methods**) is plotted as a function of the β-phase fraction ($c_\beta$). The color of each marker indicates whether the α/β-$PdH_x$ interface at that configuration is more closely aligned with the {110} or {211} orientation. **b**, Snapshots from the three representative trajectories, spanning $c_\beta \approx 0.06$ to 0.94. The first five snapshots correspond to those shown in **Figure 4c**. Black pentagram markers indicate the snapshots corresponding to the transition state.

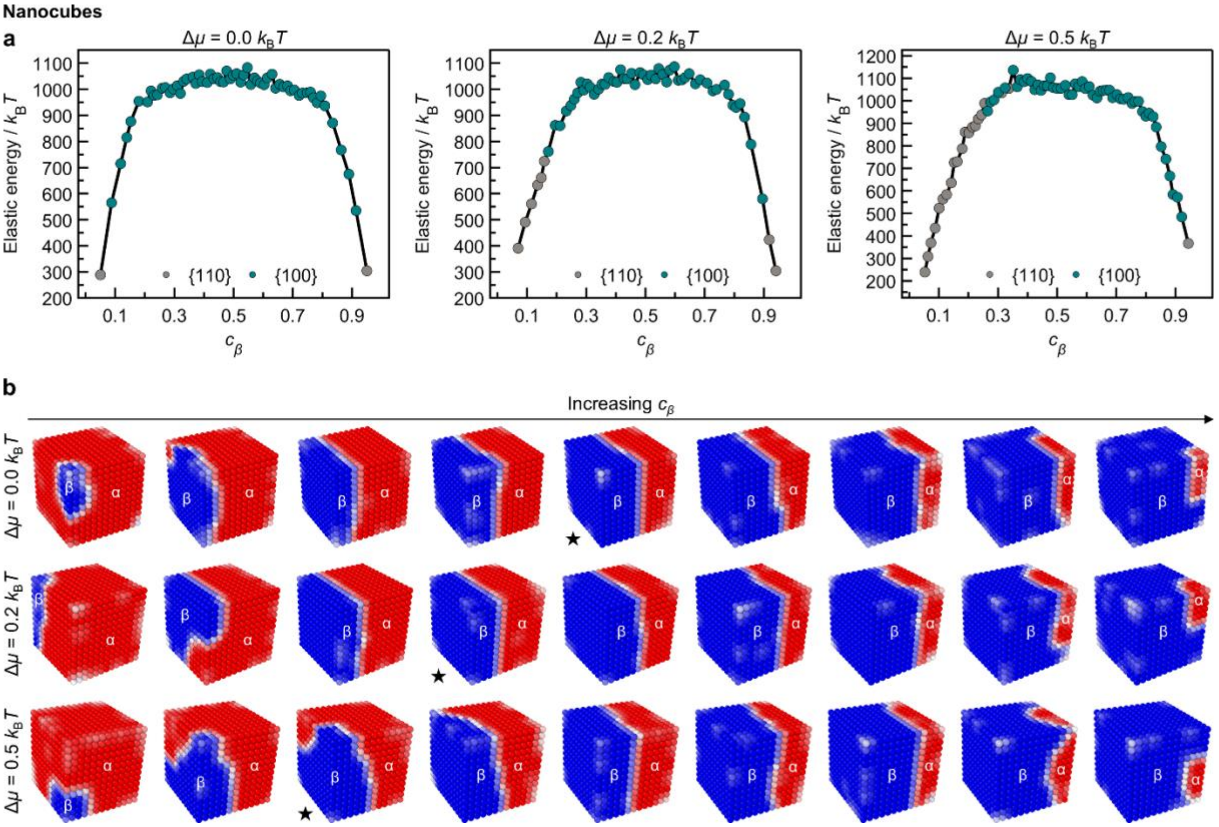


**Figure S18.** Detailed analysis of the representative hydrogenation trajectories in nanocubes. **a**, For each representative trajectory under the three chemical driving forces, $\Delta\mu$, the elastic energy (see **Methods**) is plotted as a function of the β-phase fraction ($c_\beta$). The color of each marker indicates whether the α/β-$PdH_x$ interface at that configuration is more closely aligned with the {110} or {100} orientation. **b**, Snapshots from the three representative trajectories, spanning $c_\beta \approx 0.06$ to 0.94. The first five snapshots correspond to those shown in **Figure 5c**. Black pentagram markers indicate the snapshots corresponding to the transition state.

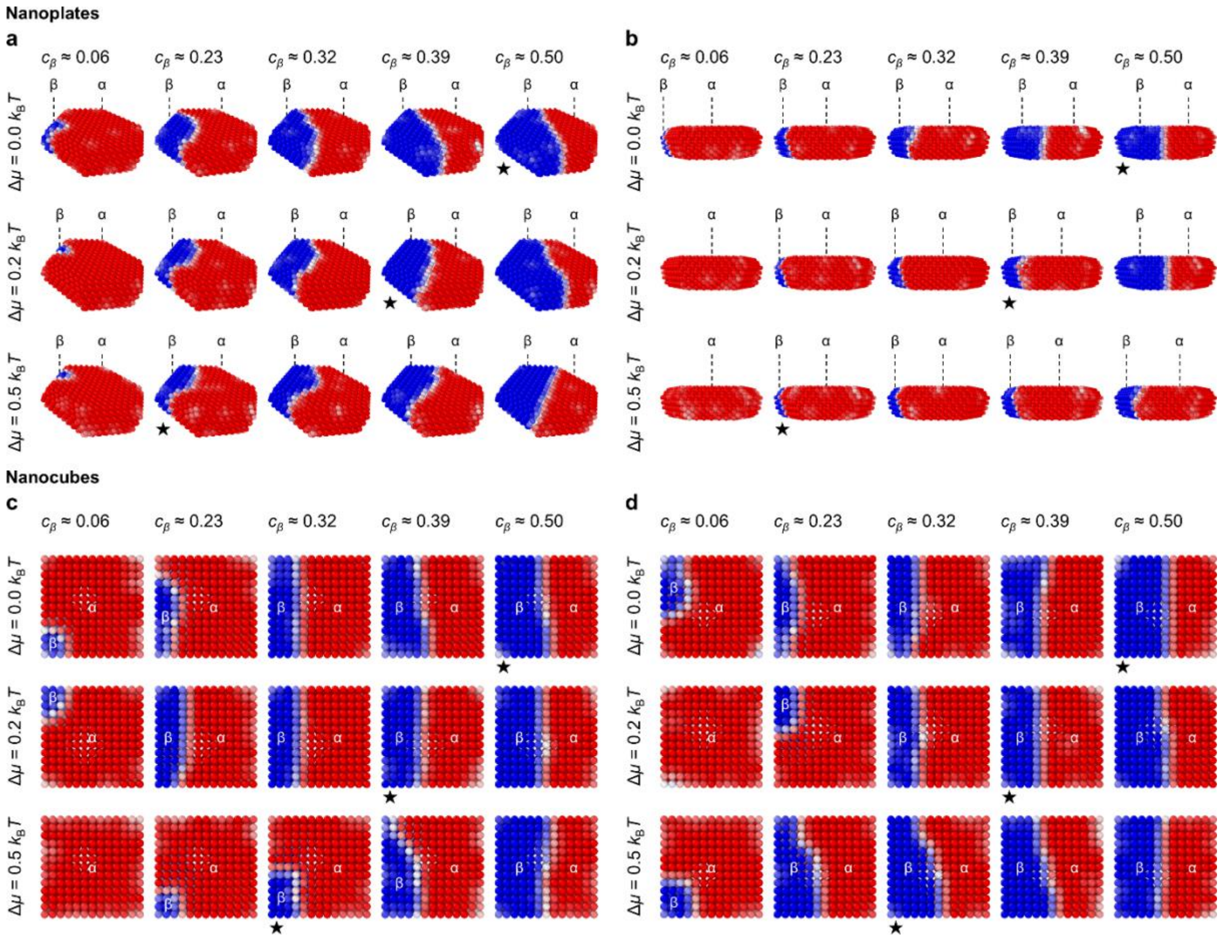


**Figure S19.** Alternative perspectives of snapshots from the representative hydrogenation trajectories in both nanocrystal geometries. **a**,**b**, The snapshots shown in **Figure 4c**, viewed from a tilted perspective (**a**) and from a side-on <211> direction (**b**). **c**,**d**, The snapshots shown in **Figure 5c**, viewed from two <100> directions orthogonal to the direction of the interface propagation. Black pentagram markers indicate the snapshots corresponding to the transition state. Please note that the $PdH_x$ phase assignments are based solely on the phases visible from the current viewing perspectives.

**Supporting Movie Legends**

**Movie S1.** *In situ* HRTEM visualization of hydrogen absorption in Nanocube.

**Movie S2.** *In situ* HRTEM visualization of hydrogen absorption in Nanoplate #1.

**Movie S3.** *In situ* HRTEM visualization of hydrogen absorption in Nanoplate #2.

**Movie S4.** *In situ* HRTEM visualization of hydrogen absorption in Nanoplate #3.

**Movie S5.** Simulated hydrogen absorption in nanoplate, propagating under $\Delta\mu = 0.0\ k_B T$.

**Movie S6.** Simulated hydrogen absorption in nanoplate, propagating under $\Delta\mu = 0.2\ k_B T$.

**Movie S7.** Simulated hydrogen absorption in nanoplate, propagating under $\Delta\mu = 0.5\ k_B T$.

**Movie S8.** Simulated hydrogen absorption in nanocube, propagating under $\Delta\mu = 0.0\ k_B T$.

**Movie S9.** Simulated hydrogen absorption in nanocube, propagating under $\Delta\mu = 0.2\ k_B T$.

**Movie S10.** Simulated hydrogen absorption in nanocube, propagating under $\Delta\mu = 0.5\ k_B T$.
